# Supplementary material for: Unsupervised Model Selection for Time-series Anomaly Detection
Source: arXiv:2210.01078 source file (2023-01-24)
Supplement: Supplementary file 1 [file A6_hyperparameters.tex]

\subsection{Hyper-parameters}
\label{a:hyperparams}

\subsubsection{Model}

\subsubsection{Synthetic Anomaly Injection}
