# Supplementary material for: Unsupervised Model Selection for Time-series Anomaly Detection
Source: arXiv:2210.01078 source file (2023-01-24)
Supplement: Supplementary file 2 [file old_A9_EI_theory.tex]

\andrey{Sorry, this section doesn't work, whether we assume Mallow's model or not. I think as M goes to infinity, empirical influence goes to zero, and ratio of influences goes to one.}


Let $[N] = \{1, 2, \cdots, N\}$ denote the universe of elements and $S_N$ be the set of permutations on $[N]$. For $\sigma \in S_N$, let $\sigma(i)$ denote the rank of element $i$. In the following section, we use rankings and permutations interchangeably. 
% and $\sigma^{-1}(j)$ denote the element at rank $j$. 

% \andrey{Difference between ranking and permutation is that permutation cannot have ties (same rank). I think you should mention that when we use surrogate metrics, we break ties uniformly at random.}

Consider $N$ anomaly detection models $A_1, \cdots, A_{N}$. Let each model be represented by an item in the set $[N]$. Also consider a set of $M$ surrogate metrics $\mathcal{S} = \{\sigma_1, \cdots \sigma_M\}$, each of which induces a ranking in $S_N$ i.e. $\sigma_i \in S_N, \ \forall i \in [M]$. In what follows, we use $\sigma_k$ to both refer to the surrogate metric and the ranking it induces. We say that a metric $\sigma_k$ prefers model $A_i$ over $A_j$ if $\sigma_k(i) < \sigma_k(j)$. A metric prefers $A_i$ over $A_j$ if it \textit{perceives} that the former is more accurate than the latter. Ties between models are broken uniformly at random. Let $\sigma^* \in S_N$ denote the true ranking of models. Without loss of generality, we assume true ranking to be the identity permutation, which maps every element of the set to itself. 

% \andrey{p needs to be defined w.r.t. surrogate measure or permutation.}

Let $p_\mathcal{S} \in \mathbb{N}^N$ denote a vector of points with respect to a set of permutations $\mathcal{S}$, such that $p_\mathcal{S}(i)$ denotes the total number of points received by item $i \in [N]$. Let $\texttt{sort}(\cdot)$ denote the sorting operator. Given any arbitrary $d$-dimensional vector $v \in \mathbb{R}^d$, $\texttt{sort}(v)$ is the vector $v$ sorted in descending order. 
% Given any arbitrary vector of points $p$ as input, $q \triangleq \texttt{sort}(p) \in \mathbb{N}^N$ is a vector with the elements of $p$ in ascending order \textit{i.e.} $q(1) \leq q(2) \leq \cdots q(N)$.  
% \andrey{Definition of sort(.) is incorrect. Sigma contains indexes 1, ..., N, rather than points. Actually, you don't need to define sort, just explain in words.}
In Borda rank aggregation, given a permutation $\sigma_j$, the $i^{th}$ item receives $N - \sigma_j(i)$ points. Then for a set of permutations $\mathcal{S}$, the $i^{th}$ item receives a total of $p_{\mathcal{S}}(i) = \sum_{\sigma_j \in \mathcal{S}} N - \sigma_j(i)$ points. Then the aggregated permutation according to the Borda method over permutations in $\mathcal{S}$ is $\hat \sigma_{\mathcal{S}} \triangleq \texttt{sort}(p_{\mathcal{S}})$.

For any two permutations $\sigma_k$ and $\sigma_l$, the Kendall's $\tau$ distance is defined as the number of pairwise disagreements: \begin{equation} d_\tau(\sigma_k, \sigma_l) = \sum_{i < j} \mathbb{I}\{(\sigma_k(i) - \sigma_k(j))(\sigma_l(i) - \sigma_l(j))<0\} \end{equation}

For some $\sigma_k\in \mathcal{S}$, empirical influence $\text{EI}(\sigma_k, \mathcal{S})$ measures the impact of $\sigma_i$ on the Borda solution. 

\begin{equation}
\text{EI}(\sigma_k, \mathcal{S})= f(\mathcal{S}) - f(\mathcal{S} \setminus \sigma_k), \quad \text{where } f(\mathcal{A}) = \frac{1}{|\mathcal{A}|} \sum_{i=1}^{|\mathcal{A}|} d_{\tau}(\text{Borda}(\mathcal{A}), \sigma_i)    
\end{equation}


Consider a set of $M$ surrogate metrics for model selection, and rankings $\sigma_k$ induced by these metrics. The degree to which each ranking $\sigma_k$ correlates with (unknown) ground truth ranking $\sigma^{\ast}$ varies. In this section, we show that the proposed Empirical Influence criterion can be used to approximate relative strength of rank correlation between $\sigma_k$ and $\sigma^{\ast}$. Informally, this means that Empirical Influence can be used as a proxy for surrogate metric "quality" without accessing the ground truth.

% We can identify bad (low probability) permutations as they are likely to have high positive empirical influence. In fact, Theorem~\ref{thm:ei} shows that empirical influence asymptotically approximates the ``\textit{quality}" of a permutation, i.e., the distance between the permutation and the ground truth. This is important because, without knowing the ground truth permutation, we cannot compute this distance, but we can compute empirical influence. We first introduce a proposition that we will later use to prove Theorem~\ref{thm:ei}.

Consider a set of $M$ permutations $\mathcal{S} = \{\sigma_1, \cdots, \sigma_M\}$, where $\sigma_i \in S_N$. Let $\hat{\sigma}_{\mathcal{S}}$ be the result of Borda aggregation applied to $\mathcal{S}$. Recall that in the Borda approach, each item to rank (i.e., each anomaly detection model) receives points and the items are then sorted in the decreasing order of points. Let $p_\mathcal{S}(i)$ be the number of points given to itme $i$ by Borda aggregation over set  $\mathcal{S}$. Before introducing our observation about Empirical Inference, we introduce an auxiliary lemma.

\begin{lemma} Assume that $\underset{i,j}{\min} \ | p_\mathcal{S}(i) - p_\mathcal{S}(j) | \geq c M$ for some $c > 0$. Then $\underset{M \xrightarrow[]{} \infty}{\lim} d_{\tau}(\hat \sigma_{\mathcal{S}}, \hat \sigma_{\mathcal{S} \setminus \sigma_k})=0$, where $d_{\tau}$ is Kendall's $\tau$ distance.
\label{prop:borda_invariance}
\end{lemma}

\begin{proof}
Consider an arbitrary item $i \in [N]$. Under the Borda method, for two sets of permutations $\mathcal{S}$ and $\mathcal{S} \setminus \sigma_k$, item $i$ receives a total of $p_{\mathcal{S}}(i) = MN - \sum _{j=1}^M \sigma_j(i)$ and $p_{\mathcal{S} \setminus k}(i) = (M-1)N -  \sum_{j=1}^M \sigma_j(i) + \sigma_k(i)$ points, respectively.

Next, consider another item $j \in [N]$ such that $j = \underset{j \in [N]}{\argmin} \ |p_\mathcal{S}(i) - p_\mathcal{S}(j)|$. Intuitively, item $j$ has the highest chance of being swapped with item $i$.

To understand whether applying Borda on either $\mathcal{S}$ or $\mathcal{S} \setminus \sigma_k$ will result in different rankings, we consider the quantity $\lim _{M \to \infty} \frac{|p_{\mathcal{S}}(i) - p_{\mathcal{S} \setminus k}(i)|}{|p_\mathcal{S}(i) - p_\mathcal{S}(j)|}$: 
\begin{align*}
    \frac{|p_{\mathcal{S}}(i) - p_{\mathcal{S} \setminus k}(i)|}{ |p_\mathcal{S}(i) - p_\mathcal{S}(j)|} & = \frac{|MN - \sum _{j=1}^M \sigma_j(i) -\left( (M-1) N - \sum_{j=1}^M \sigma_j(i) + \sigma_k(i)\right)|}{ |p_\mathcal{S}(i) - p_\mathcal{S}(j)|} \\
    & = \frac{|N  - \sigma_k(i)|}{ |p_\mathcal{S}(i) - p_\mathcal{S}(j)| } \\
    & \leq \frac{|N  - \sigma_k(i)|}{cM}
\end{align*}

Hence, $\lim _{M \to \infty} \frac{|p_{\mathcal{S}}(i) - p_{\mathcal{S} \setminus k}(i)|}{|p_\mathcal{S}(i) - p_\mathcal{S}(j)|} = 0$

As $M \to \infty$, the difference in points using $\mathcal{S}$ or $\mathcal{S} \setminus \sigma_k$ relative to the difference in points given to any two items tends to zero. Therefore, $\underset{M \xrightarrow[]{} \infty}{\lim} d_{\tau}(\hat \sigma_{\mathcal{S}}, \hat \sigma_{\mathcal{S} \setminus \sigma_k})=0$.

%Intuitively, removing a permutation does not create a significant difference in points so as to change the Borda aggregation solution, as the number of permutations increases. Since our arguments are true for all items $i \in [N]$, asymptotically as $M \xrightarrow[]{} \infty$, $p_{\mathcal{S}}(i) = p_{\mathcal{S} \setminus \sigma_k}(i) \implies \texttt{sort}(p_{\mathcal{S}}) = \texttt{sort}(p_{\mathcal{S} \setminus \sigma_k}) \implies \hat \sigma_{\mathcal{S}} = \hat \sigma_{\mathcal{S} \setminus \sigma_k}$
\end{proof}

\begin{theorem} Consider an arbitrary infinite sequence of permutations $\sigma_1,\sigma_2,\ldots$ over $N$ items and a sequence of subsets $\mathcal{S}(M)=\{\sigma_i\}_{i=1}^M$. Given $\mathcal{S}$(M), choose arbitrary $\sigma_i(M),\sigma_j(M)\in\mathcal{S}(M)$. In the notation below, we omit dependency on M for brevity.

Under the same assumptions as in Lemma~\ref{prop:borda_invariance}, we have that $\underset{M \to \infty}{\lim} \frac{\text{EI}(\sigma_i, \mathcal{S})}{\text{EI}(\sigma_j, \mathcal{S})}  = \frac{d_{\tau}(\hat \sigma_{\mathcal{S}}, \sigma_i)}{d_{\tau}(\hat \sigma_{\mathcal{S}}, \sigma_j)}$, where EI is the Empirical Influence. 
\label{thm:ei}
\end{theorem}
\begin{proof}
We start with the definition of the Empirical Influence

\begin{align*}
    \text{EI}(\sigma_i, \mathcal{S})
    &=\frac{1}{M}\sum_{\sigma_a \in \mathcal{S}} d_\tau(\hat \sigma_{\mathcal{S}}, \sigma_a) - \frac{1}{M-1}\sum_{\sigma_b \in \mathcal{S} \setminus \sigma_i} d_\tau(\hat \sigma_{\mathcal{S} \setminus \sigma_i}, \sigma_b) \\
    &=\frac{1}{M} \left( d_\tau(\hat \sigma_{\mathcal{S}}, \sigma_i) +  \sum_{\sigma_a \in \mathcal{S} \setminus \sigma_i} d_\tau(\hat \sigma_{\mathcal{S}}, \sigma_a) - \frac{M}{M-1}\sum_{\sigma_b \in \mathcal{S} \setminus \sigma_i} d_\tau(\hat \sigma_{\mathcal{S} \setminus \sigma_i}, \sigma_b) \right) \\
    &=\frac{1}{M} \left( d_\tau(\hat \sigma_{\mathcal{S}}, \sigma_i) +  \sum_{\sigma_a \in \mathcal{S} \setminus \sigma_i}  \left( d_\tau(\hat \sigma_{\mathcal{S}}, \sigma_a) - \frac{M}{M-1} d_\tau(\hat \sigma_{\mathcal{S} \setminus \sigma_i}, \sigma_a) \right) \right)
\end{align*}

We have that
\begin{align*}
    \frac{\text{EI}(\sigma_i, \mathcal{S})}{\text{EI}(\sigma_j, \mathcal{S})}
    = \frac
    {d_\tau(\hat \sigma_{\mathcal{S}}, \sigma_i) +  \sum_{\sigma_a \in \mathcal{S} \setminus \sigma_i}  \left( d_\tau(\hat \sigma_{\mathcal{S}}, \sigma_a) - \frac{M}{M-1} d_\tau(\hat \sigma_{\mathcal{S} \setminus \sigma_i}, \sigma_a) \right) }
    {d_\tau(\hat \sigma_{\mathcal{S}}, \sigma_j) +  \sum_{\sigma_a \in \mathcal{S} \setminus \sigma_j}  \left( d_\tau(\hat \sigma_{\mathcal{S}}, \sigma_a) - \frac{M}{M-1} d_\tau(\hat \sigma_{\mathcal{S} \setminus \sigma_j}, \sigma_a) \right) }
\end{align*}

Next, consider the term

\begin{align*}
    \left( d_\tau(\hat \sigma_{\mathcal{S}}, \sigma_a) - \frac{M}{M-1} d_\tau(\hat \sigma_{\mathcal{S} \setminus \sigma_j}, \sigma_a) \right)
    \leq d_\tau(\hat \sigma_{\mathcal{S}}, \sigma_a)
\end{align*}

Kendall's $\tau$ is a metric, hence

\begin{align*}
    \sum_{\sigma_a \in \mathcal{S} \setminus \sigma_i}  \left( 0 - \frac{M}{M-1} d_\tau(\hat \sigma_{\mathcal{S} \setminus \sigma_i}, \sigma_a) \right) \\
    \leq \sum_{\sigma_a \in \mathcal{S} \setminus \sigma_i}  \left( d_\tau(\hat \sigma_{\mathcal{S}}, \sigma_a) - \frac{M}{M-1} d_\tau(\hat \sigma_{\mathcal{S} \setminus \sigma_i}, \sigma_a) \right) \\
    \leq     \sum_{\sigma_a \in \mathcal{S} \setminus \sigma_i}
    \left(
        d_\tau(\hat \sigma_{\mathcal{S}}, \hat \sigma_{\mathcal{S} \setminus \sigma_i})
        + d_\tau(\hat \sigma_{\mathcal{S} \setminus \sigma_i}, \sigma_a)
        - \frac{M}{M-1} d_\tau(\hat \sigma_{\mathcal{S} \setminus \sigma_i}, \sigma_a)
    \right) \\
    = \sum_{\sigma_a \in \mathcal{S} \setminus \sigma_i}
    \left(
        d_\tau(\hat \sigma_{\mathcal{S}}, \hat \sigma_{\mathcal{S} \setminus \sigma_i})
        - \frac{1}{M-1} d_\tau(\hat \sigma_{\mathcal{S} \setminus \sigma_i}, \sigma_a)
    \right) \\
\end{align*}

no proof
% \begin{align*}
%     \lim_{M \to \infty}\frac{\text{EI}(\sigma_i, \mathcal{S})}{\text{EI}(\sigma_j, \mathcal{S})} & = \lim_{M \to \infty} \frac{\frac{1}{M}\sum_{\sigma_k \in \mathcal{S}} d_\tau(\hat \sigma_{\mathcal{S}}, \sigma_k) - \frac{1}{M-1}\sum_{\sigma_k \in \mathcal{S} \setminus \sigma_i} d_\tau(\hat \sigma_{\mathcal{S} \setminus \sigma_i}, \sigma_k)}{\frac{1}{M}\sum_{\sigma_k \in \mathcal{S}} d_\tau(\hat \sigma_{\mathcal{S}}, \sigma_k) - \frac{1}{M-1}\sum_{\sigma_k \in \mathcal{S} \setminus \sigma_j} d_\tau(\hat \sigma_{\mathcal{S} \setminus \sigma_j}, \sigma_k)} \\
%     & = \lim_{M \to \infty} \frac{\frac{1}{M}d_\tau(\hat \sigma_{\mathcal{S}}, \sigma_i) + \left( \frac{\sum_{\sigma_k \in \mathcal{S}} d_\tau(\hat \sigma_{\mathcal{S}}, \sigma_k)}{M} - \frac{\sum_{\sigma_k \in \mathcal{S} \setminus \sigma_i} d_\tau(\hat \sigma_{\mathcal{S} \setminus \sigma_i}, \sigma_k)}{M-1} \right)}{\frac{1}{M}d_\tau(\hat \sigma_{\mathcal{S}}, \sigma_j) + \left( \frac{\sum_{\sigma_k \in \mathcal{S}} d_\tau(\hat \sigma_{\mathcal{S}}, \sigma_k)}{M} - \frac{\sum_{\sigma_k \in \mathcal{S} \setminus \sigma_i} d_\tau(\hat \sigma_{\mathcal{S} \setminus \sigma_j}, \sigma_k)}{M-1} \right)} \\
%     & = \lim_{M \to \infty} \frac{d_\tau(\hat \sigma_{\mathcal{S}}, \sigma_i) + \left( \sum_{\sigma_k \in \mathcal{S}} d_\tau(\hat \sigma_{\mathcal{S}}, \sigma_k) - \frac{M}{M-1}\sum_{\sigma_k \in \mathcal{S} \setminus \sigma_i} d_\tau(\hat \sigma_{\mathcal{S} \setminus \sigma_i}, \sigma_k) \right)}{d_\tau(\hat \sigma_{\mathcal{S}}, \sigma_j) + \left( \sum_{\sigma_k \in \mathcal{S}} d_\tau(\hat \sigma_{\mathcal{S}}, \sigma_k) - \frac{M}{M-1} \sum_{\sigma_k \in \mathcal{S} \setminus \sigma_i} d_\tau(\hat \sigma_{\mathcal{S} \setminus \sigma_j}, \sigma_k) \right)} \\
%     & \text{Using Proposition~\ref{prop:borda_invariance} and } \lim_{M \to \infty} \frac{M}{M-1} = 1: \\
%     & = \frac{d_\tau(\hat \sigma_{\mathcal{S}}, \sigma_i)}{d_\tau(\hat \sigma_{\mathcal{S}}, \sigma_j)}
% \end{align*}
\end{proof}

\paragraph{Definition.} The Mallows's model is a popular distance-based distribution to model rank data. The probability mass function of a Mallows's model $\mathcal{M}(\sigma_0, \theta)$ with central permutation $\sigma_0$ and dispersion parameter $\theta$ is given by: 
$$p(\sigma) = \frac{exp(-\theta d(\sigma, \sigma_0))}{\psi}$$ where $d$ is the Kendall's $\tau$ distance. 


\begin{corollary}
If $\sigma_1, \cdots, \sigma_M \sim \mathcal{M}(\sigma_0, \theta)$, then $\underset{M \to \infty}{\lim} \frac{\text{EI}(\sigma_i, \mathcal{S})}{\text{EI}(\sigma_j, \mathcal{S})}  = \frac{d(\sigma_i, \sigma_{0})}{d(\sigma_j, \sigma_{0})}$.
\end{corollary}
\begin{proof}
The proof follows from the fact that as $M \to \infty$ Borda recovers the location parameter of the Mallows model $\sigma_0$, due to \citep{fligner1986distance}.
\end{proof}


Intuitively, if all the permutations are drawn from a Mallows distribution, then empirical influence identifies low probability permutations. Recall that for permutations drawn from a mallows distribution with central permutation $\sigma_0$, low probability permutations have high kendall's $\tau$ distance from $\sigma_0$.
